# Supplementary material for: Ads Recommendation in a Collapsed and Entangled World
Source: arXiv:2403.00793 source file (2024-07-05)
Supplement: Supplementary file 1 [file 11.appendix.tex]

\newpage
\section{Appendix}
\subsection{Exploration with Uncertainty Estimates}
\label{appendix: exploration}
\subsubsection{Gaussian Process for CTR prediction}

A GP prior distribution assumption over $f \sim \mathcal{GP}(m_{\theta}(\mathbf{x}), k_{\theta}(\mathbf{x}, \mathbf{x}^\prime))$ where $m(\mathbf{x}) = \mathbb{E}[f(\mathbf{x})]$ denotes the mean function and $k_{\theta}(\mathbf{x}, \mathbf{x}^\prime) = \mathbb{E}[(f(\mathbf{x}) - m(\mathbf{x}))(f(\mathbf{x}^\prime) - m(\mathbf{x}^\prime))]$ denotes the covariance function in which $\mathbf{x}$ and $\mathbf{x}^\prime$ denote different input locations where the function $f$ is evaluated, and $\theta$ denotes the set of hyperparameters of the kernel functions. A common choice for the mean function is $m(\mathbf{x})=0$ (since the prior knowledge and uncertainty about the mean function can be taken into account by adjusting the kernel function). 

After accounting for the mean function, the GP is fully specified by the form of the covariance/kernel function and the associated hyperparameters $\theta$.

The task typically involves predicting the latent function value $f^{\star} = f(\mathbf{x}^{\star})$ at an unseen test input $\mathbf{x}^{\star}$. Let  $\mathbf{X} \triangleq \{\mathbf{x}_n\}_{n=1}^{N}$ denotes the training data inputs, $\mathbf{f} \triangleq \{f(\mathbf{x}_n)\}_{n=1}^{N}$ represents the latent function values, and $\mathbf{y} \triangleq \{y_n\}_{n=1}^{N}$ be the user feedback (click or not). Here each feedback $y_n$ is corrupted as a noisy measurement of latent function values $f(\mathbf{x}_n)$ by a Bernoulli likelihood $p(y_n|f(\mathbf{x}_n)) = \mathrm{Ber}(y_n; \sigma(f(\mathbf{x}_n))$ where $\sigma(\cdot)$ corresponds to the sigmoid function. Then the joint distribution of $\{f^{\star}, \mathbf{f}, \mathbf{y}\}$ can be written as $p(f^{\star}, \mathbf{f}, \mathbf{y}) = p(f^{\star}, \mathbf{f})p(\mathbf{y}|\mathbf{f})$
and $p(\mathbf{y}|\mathbf{f}) = \prod\limits_{n=1}^{N}\mathrm{Ber}(y_n; \sigma(f(\mathbf{x}_n))$. The joint distribution $p(f^{\star}, \mathbf{f})$ can be represented with a multivariate normal distribution:
    \begin{equation}
        \begin{bmatrix}
            f^\star
            \\
            \mathbf{f}
        \end{bmatrix}
        \sim
        \mathcal{N}\left(
            \begin{bmatrix}
                0
                \\
                \mathbf{0}
            \end{bmatrix}
            ,
            \begin{bmatrix}
                k_{\mathbf{x}^{\star}\mathbf{x}^{\star}} & \mathbf{k}_{\mathbf{x}^{\star}\mathbf{X}}
                \\
                \mathbf{k}_{\mathbf{X}\mathbf{x}^{\star}} & \mathbf{K}_{\mathbf{X}\mathbf{X}}
            \end{bmatrix}
        \right)
    \end{equation}
    
   where $k_{\mathbf{x}^\star\mathbf{x}^\star} = k_{\theta}(\mathbf{x}^\star, \mathbf{x}^\star)$ is the variance of the test function value, $\mathbf{k}_{\mathbf{x}^\star\mathbf{X}} \triangleq \mathbf{k}_{\mathbf{X}\mathbf{x}^\star}^\top$ and $\mathbf{k}_{\mathbf{x}^\star\mathbf{X}}$ denotes a vector with components $k_{\theta}(\mathbf{x}^\star, \mathbf{x}_n)$ for $n = 1, 2, \dots, N$. $\mathbf{K}_{\mathbf{X}\mathbf{X}}$ denotes the covariance matrix with components $k_{\theta}(\mathbf{x}_n, \mathbf{x}_{n^\prime})$ for $n, n^\prime = 1, 2, \dots, N$. 

    Therefore, the posterior distribution of $f^{\star}$ given observations $\mathbf{y}$ can be rewritten as: $p(f^{\star}|\mathbf{y}) = 1/p(\mathbf{y}) \int p(\mathbf{y}|\mathbf{f})p(f^{\star}, \mathbf{f}) \mathrm{d}\mathbf{f}$.

   This suggests that the predictive distribution of the function value at an unseen test input is Gaussian-distributed with the posterior mean and variance. In this regard, a GP can been seen as a prior over the function $f$. Conditioning this prior on the training data results in a posterior that 'fits' the data. Please refer to \citet{williams2006gaussian} for more details.

% \subsection{Feature Correlation}

% We present such semantic-temporal correlation in our production dataset in Fig.~\ref{fig:stc}.
% In particular, we pick up a target category \texttt{A}, and calculate the ground-truth correlation of behaviors belonging to various categories (\texttt{A} to \texttt{J} along the y-axis) with different time intervals or at relative positions regarding the target.
% Among all history behaviors, those belonging to the same category with the target, \textit{i.e.}, the 1st row in both figures, are more correlated to the user's response on target.
% In addition, there is a strong time-decaying pattern among these behaviors of the category \texttt{A}, that is, those close to the target temporally are more informative.
% Such a decaying pattern is more strong on time intervals than relative position.
% % \cmt{More definition and examples.}

% \begin{figure}[!htb]
%     \centering
%     \begin{tabular}{c}
%             % \includegraphics[width=0.48\textwidth]{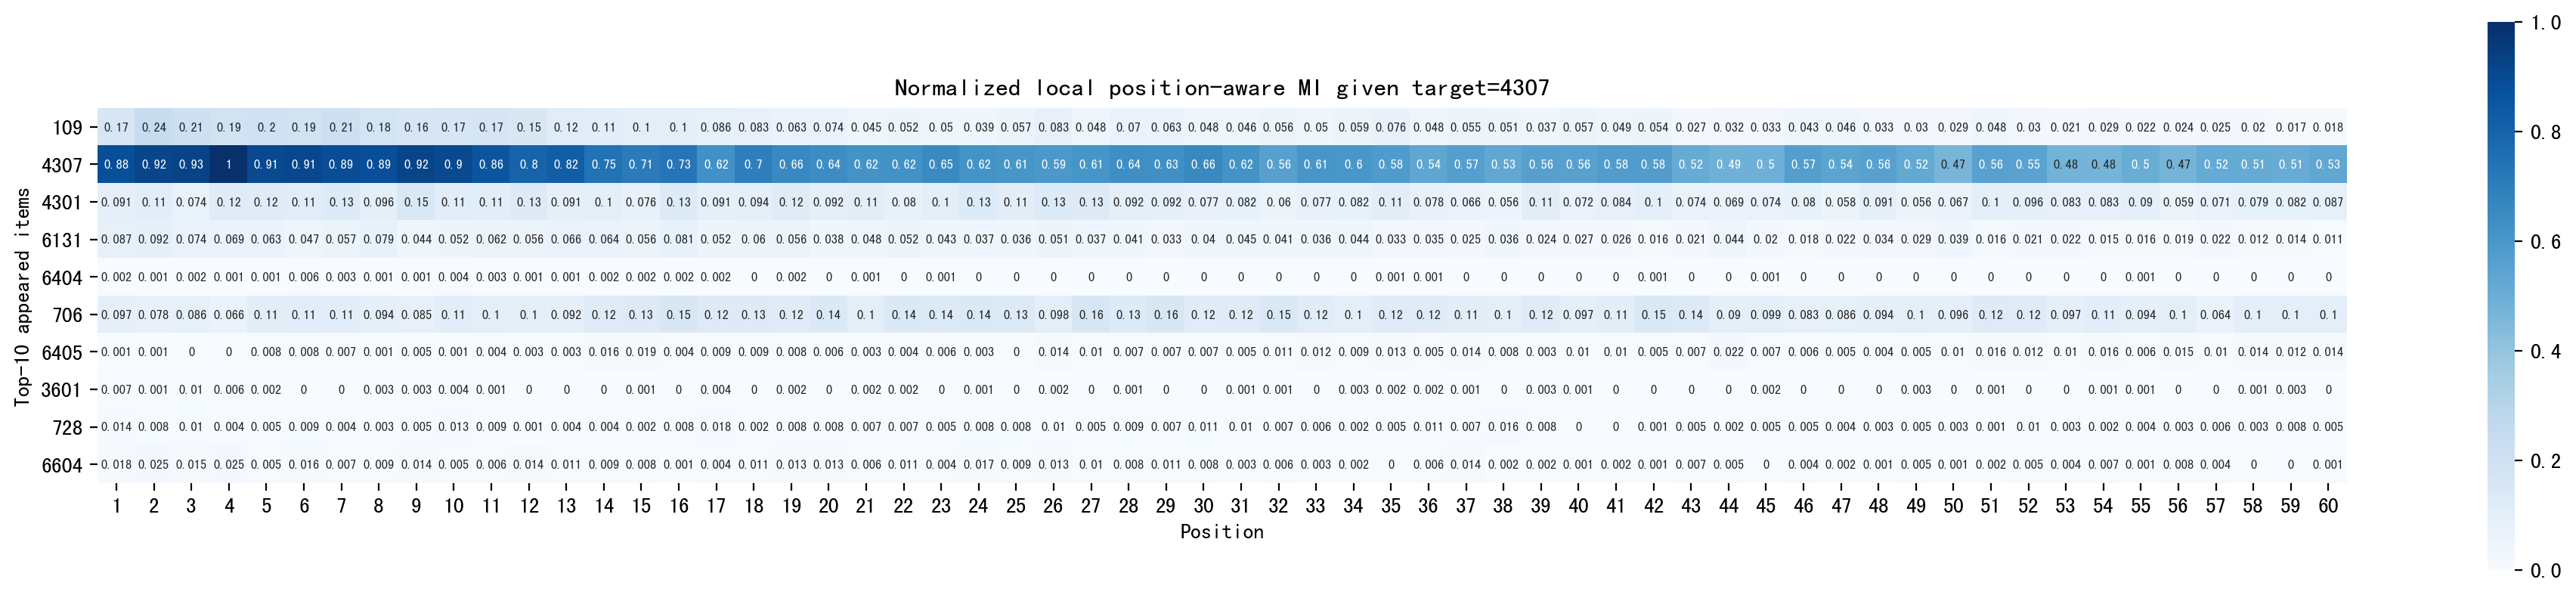} \\
%             % \includegraphics[width=0.48\textwidth]{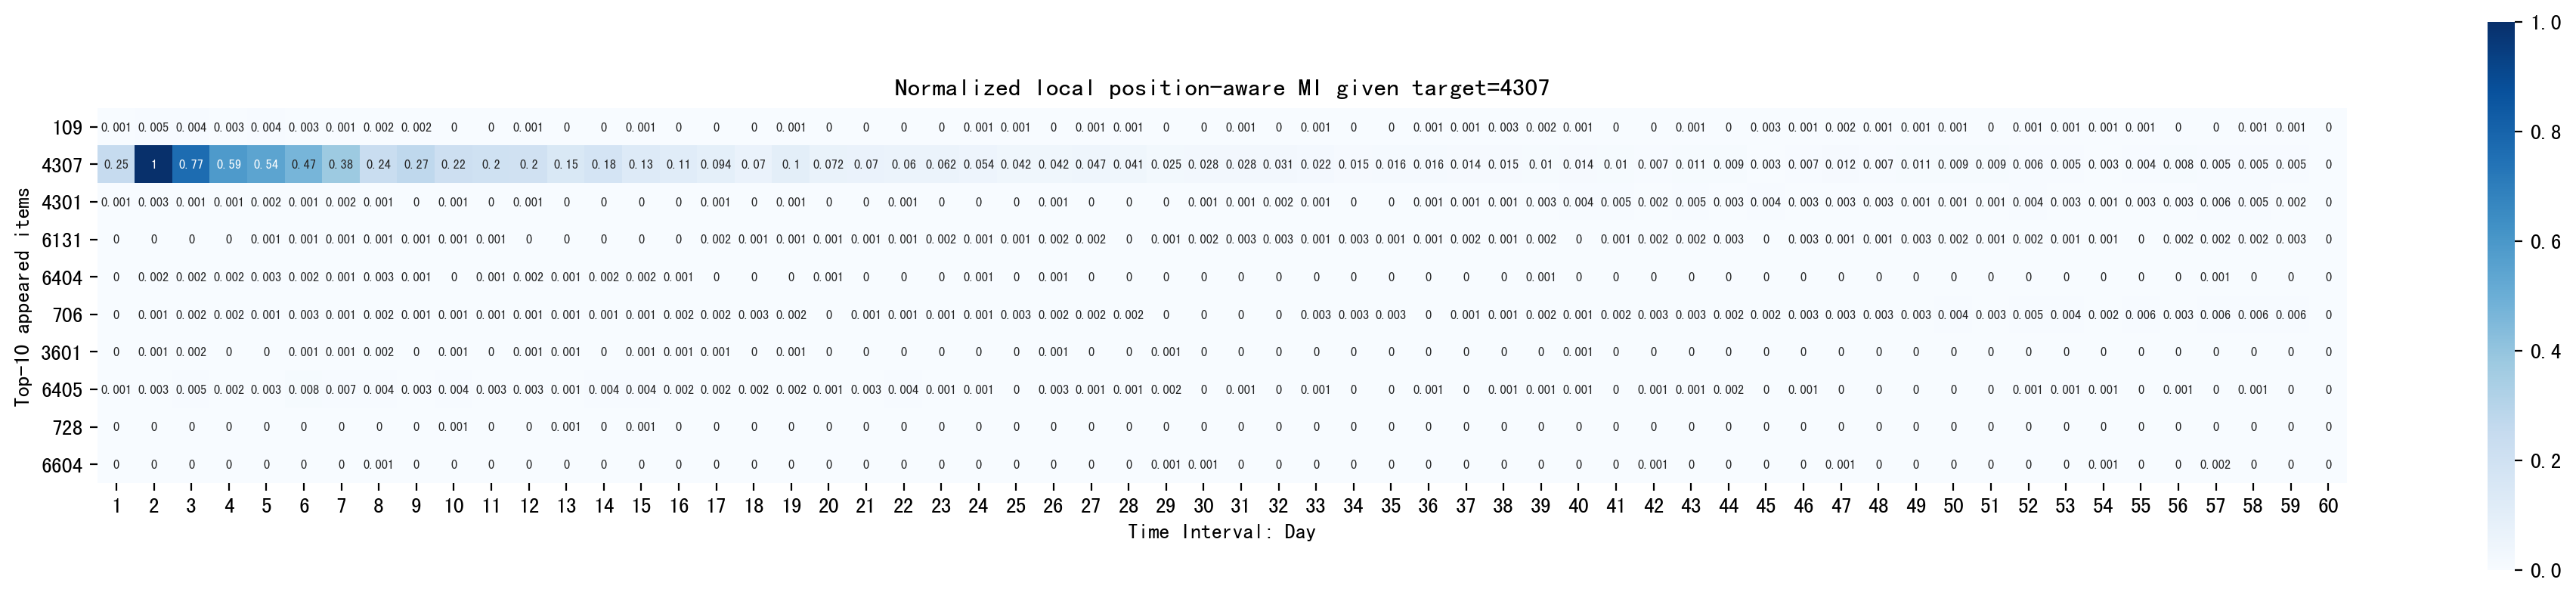}
%             \includegraphics[width=0.45\textwidth]{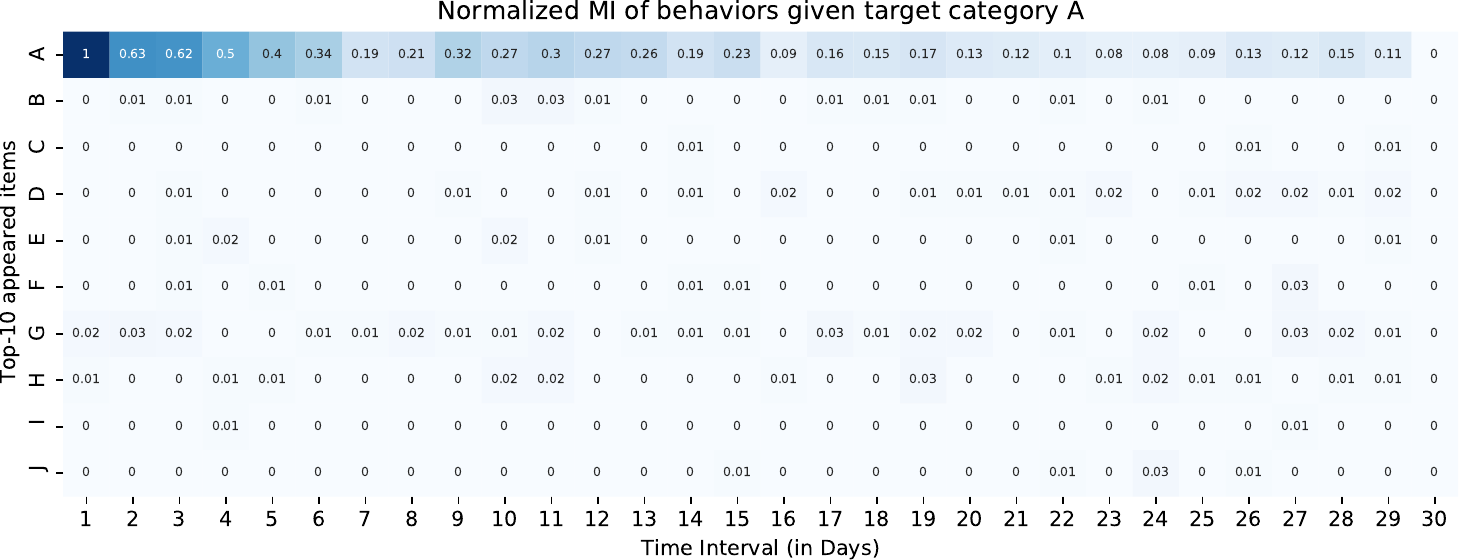} \\
%             \includegraphics[width=0.45\textwidth]{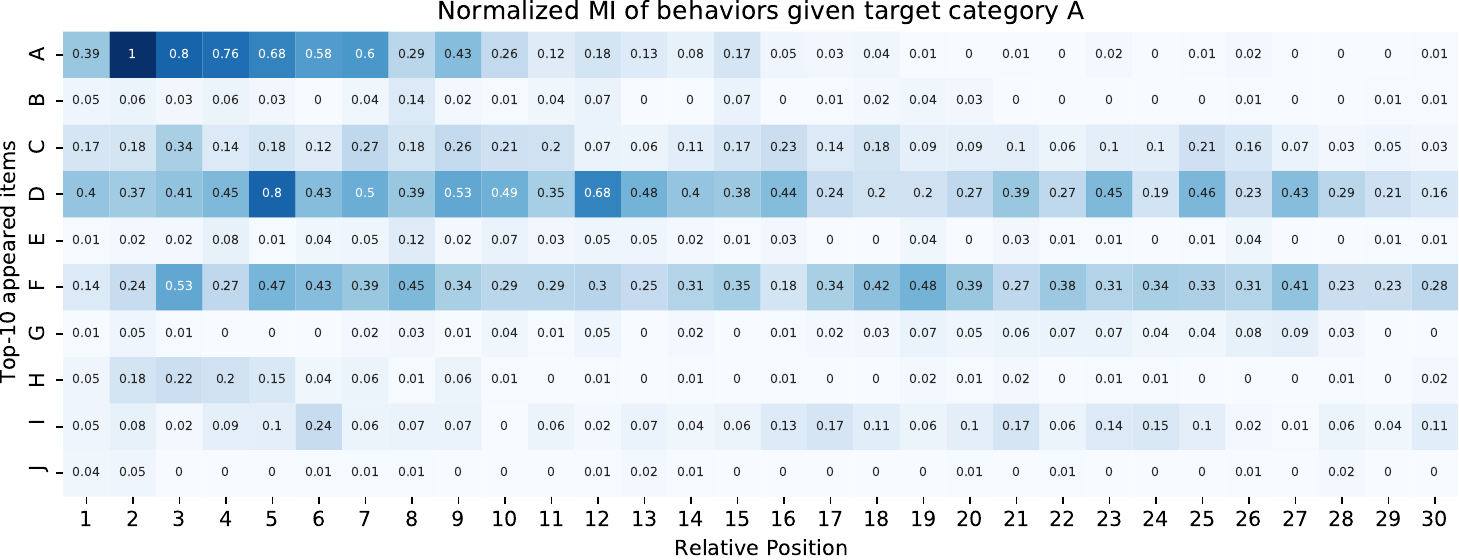}
%     \end{tabular}
%     \caption{Semantic-temporal correlation on real-world datasets}
%     \label{fig:stc}
% \end{figure}

\subsection{GwPFM}
\label{subsec:appendix_GwPFM}

\begin{align}
    \Phi_{\text{FM}} &= \sum_{i=1}^{N}\sum_{j=i+1}^N x_{i}x_{j} \langle \bm{v}_{i}, \bm{v}_{j}\rangle \\             
    \Phi_{\text{FFM}} &= \sum_{i=1}^N \sum_{j=i+1}^N x_{i} x_{j} \langle \bm{v}_{i,F(j)} , \bm{v}_{j,F(i)} \rangle \\   
    \Phi_{\text{FwFM}} &= \sum_{i=1}^N \sum_{j=i+1}^N x_{i} x_{j} \langle \bm{v}_i, \bm{v}_j\rangle r_{F(i), F(j)} \\
    \Phi_{\text{GwPFM}} &= \sum_{i=1}^N \sum_{j=i+1}^N x_{i} x_{j} \langle \bm{v}_{i,P(j)} , \bm{v}_{j,P(i)} \rangle r_{G(i), G(j)}
    % \Phi_{\text{FmFM}}(\Omega, \bm{x}) &= w_0 + \sum_{i=1}^N x_i w_i + \sum_{i=1}^N \sum_{j=i+1}^N x_{i} x_{j} ( \bm{v}_i  W_{F(i), F(j)}) \odot \bm{v}_j 
\end{align}

During online inference, we can first average pooling the input feature embeddings by groups.
Then for a given request and $C$ candidate ads, the interactions between the groups of the first part can be only calculated once, while the interactions between the first and the second part, as well as interactions within the second part need to be calculated $C$ times, one for each candidate ad.
The computation complexity is $O(N_1 P K + N_2 P C K  + \binom{G}{2} K + G F_2 K + F_2 \binom{F_2}{2} C K)$
where $N_1$ and $N_2$ denote the number of non-zero features belonging to Part 1 and Part 2, respectively, $P$ denotes the number of parts, $G$ denotes the number of feature groups in Part 1, and $K$ denotes the embedding dimension.
